# Supplementary material for: Synthetic Image Oversampling for Rare-Class Representation Learning in Deep Facial Phenotyping
Source: arXiv:2610.23730 source file (2026-11-13)
Supplement: Supplementary file 1 [file appendix.tex]

\newpage
\appendices
\section{Complete Classification Results}


\input{liao_manuscript/tables/overallresults}

\FloatBarrier

\section{Class-Weighting Sensitivity Analysis}

\input{liao_manuscript/tables/classweightablation}

\FloatBarrier

\section{GestaltMatcher-Arc Embedding Analysis}


\input{liao_manuscript/tables/arcembedding}
